# Supplementary material for: Semantic Attention Flow Fields for Monocular Dynamic Scene Decomposition
Source: arXiv:2303.01526 source file (2023-09-29)
Supplement: Supplementary file 1 [file appendix.tex]

This document contains a related work comparison table (\Cref{sec:relatedwork_expanded}), details and rationale for our dataset construction (\Cref{sec:dataset}), justification of design choices throughout the approach (\Cref{sec:designchoices}), and implementation details (\Cref{sec:implementation}). Given the numerous figures and tables, many sections begin on a new page for easier reading.

Further, we include a supplemental website that highlights key findings and allows comparison between different methods and ablations for the different \titlename volumes. Please find it here: \href{https://visual.cs.brown.edu/saff}{https://visual.cs.brown.edu/saff}

{
\begin{table*}[b]
    \centering

    \newcommand{\yes}{\ding{51}}
    \newcommand{\no}{\ding{53}}
    \newcommand{\notapplicable}{N/A}
    
    \caption{
        An comparison of related work in scene decomposition shows the unstudied area of real-world dynamic 3D segmentation without explicit segmentation clues. We investigate whether saliency can provide similar clues for the monocular video case. From this table, the closest related method is N3F; however, they take user input to define their segmentation.
       \\
        Learning: Large-scale training data:\\
        T: Supervised task-specific data.\\
        P: Generic features (e.g., ImageNet).\\
        \no: No features used.
        \label{tab:relatedwork_expanded}
    }
    %\resizebox{\linewidth}{!}{
    \begin{tabular}{l c c c  c c c c c }
    
    \toprule
    {} & \multirowcell{2}{Dynamic\\(video)} &
    \multirowcell{2}{Monocular} &
    \multirowcell{2}{Real\\world} & \multirowcell{2}{3D} & \multirowcell{2}{No seg. \\clue} &
    \multirowcell{2}{Learning} & 
    \multirowcell{2}{Adaptive \\ \# objects} &
    \multirowcell{2}{Object-\\level}\\
    \\
    \midrule
    
    IODINE\cite{greff2019multiobject} & \no & \yes & \no & \no & \yes & \no & \no & \yes\\
    MONET\cite{burgess2019monet} & \no & \yes & \no & \no & \yes & \no & \no & \yes\\
    Slot Attention\cite{locatello2020object} & \no & \yes & \no & \no & Mask & T & \no & \yes\\
    
    \midrule
    
    SIMONe\cite{Kabra2021SIMONeVT} & \yes & \yes & \no & \no & \yes & \no & \no & \yes\\
    SAVi\cite{kipf2022conditional} & \yes & \yes & \no & \no & Mask & T & \no & \yes\\
    SAVi++\cite{elsayed2022savipp} & \yes & \yes & \yes & \no & Mask & T & \no & \yes\\
    
    \midrule
    
    ObSuRF\cite{stelzner2021decomposing} & \no & \no & \no & \yes & \yes & \no & \no & \yes\\
    uORF\cite{yu2022unsupervised}& \no & \no & \no & \yes & \yes & \no & \no & \yes\\
    COLF\cite{smith2022colf} & \no & \no & \no & \yes & \yes & \no & \no & \yes\\
    
    \midrule
    
    PNF\cite{Kundu_2022_CVPR} & \yes & \yes & \yes & \yes & Mask & \no & \no & \yes \\
    %Panoptic-NeRF \cite{fu2022panoptic} & \yes & \yes & \yes & \no\\
    Object-NeRF \cite{yang2021objectnerf} & \no & \no & \yes & \yes & Mask & \no & \no & \yes\\
    
    \midrule
    DFF\cite{kobayashi2022distilledfeaturefields} & \no & \no & \yes & \yes & User & P & \yes & \yes\\
    N3F\cite{tschernezki22neural} & \yes & \yes & \yes & \yes & User & P & \yes & \yes\\
    
    \midrule
    ProposeReduce\cite{lin2021video} & \yes & \yes & \yes & \no & \yes & T & \yes & \yes\\
    NSFF\cite{li2020neural} & \yes & \yes & \yes & \yes & Mask & \no & \notapplicable & \notapplicable\\
    D$^2$NeRF\cite{wu2022ddnerf} & \yes & \yes & \yes & \yes & \yes & \no & \notapplicable & \notapplicable\\
    \midrule
    \titlename (this paper) & \yes & \yes & \yes & \yes & \yes & P & \yes & \yes\\
    
    \bottomrule
    
    \end{tabular}
    %}
\end{table*}
}

\newpage % new column
\section{Related Work Table}
\label{sec:relatedwork_expanded}

We include a table of related work (\cref{tab:relatedwork_expanded}). This includes work in 2D image object-centric learning (IODINE~\cite{greff2019multiobject}, MONET~\cite{burgess2019monet}, Slot Attention~\cite{locatello2020object}), 2D videos (SIMONe~\cite{Kabra2021SIMONeVT}, SAVi~\cite{kipf2022conditional}), a method that considers light field input (COLF~\cite{smith2022colf}), and works that add semantic information to fields (PNF~\cite{Kundu_2022_CVPR}) including from mask supervision (Object-NeRF~\cite{yang2021objectnerf}).

\clearpage
\section{\dataname Creation}
\label{sec:dataset}

To perform experiments on segmentations, we manually annotate object masks for every view and time step in the NVIDIA Dynamic Scene Dataset\cite{Yoon_2020_CVPR} and in the DyCheck dataset~\cite{gao2022dynamic}. Some object masks are visualized in \cref{fig:data annotate}.

One natural question is why we do not use existing unsupervised video segmentation benchmarks like DAVIS~\cite{Caelles_arXiv_2019} for evaluation. 
When testing these videos, we found that there is little camera motion in most of these videos. This causes classic structure-from-motion approaches like COLMAP~\cite{schoenberger2016sfm} to fail to estimate camera poses, thus we cannot optimize \titlename on these sequences. Concurrent tangential work attempts to improve this situation with better pose estimation~\cite{kopf2021robust, lin2021barf, zhang2022structure}.

Further, even if we did have poses, there could be no evaluation of the sequences in a 3D sense because the scenes were only ever captured with a single camera. While collecting ground truth 3D segmentation for dynamic casual videos is difficult, as discussed in the main paper, our approach allows evaluation at novel spacetime views as the scene was initially captured with 12 cameras. This gives a sense of the ability of the method to perform consistent 3D segmentation of the dynamic scene as captured by a simulated monocular camera view (main paper, Sec,~4, paragraph `Data').

We additionally mask five sequences within the DyCheck dataset~\cite{gao2022dynamic}. These are captured from a single smartphone RGB camera, and so do not have large disparity from frame to frame but may have large motion. Hold-out images can be taken by not processing some images in the videos, but these require less significant interpolation ability to render novel spacetime views.

\paragraph{Different Data}
Data in different modalities like infrared or depth data are beyond the scope of our work, but better depth information through, say, time of flight imaging would be a valuable addition to monocular reconstruction.

\newpage % new column
{
\begin{figure}[t]
    \centering
    \setlength{\tabcolsep}{1pt}
    
    % Set figure images paths for sequences
    % \newcommand{\figSeqJumping}{fig/fig_foreground/jumping}
    \newcommand{\figSeqBalloon}{fig/fig_anno/balloon}
    \newcommand{\figSeqBalloonw}{fig/fig_anno/balloon2}
    \newcommand{\figSeqDynamicFace}{fig/fig_anno/dynamicFace}
    \newcommand{\figSeqJumping}{fig/fig_anno/jumping}
    \newcommand{\figSeqSkating}{fig/fig_anno/skating}
    
    \newcommand{\figSeqTruck}{fig/fig_anno/truck}
    \newcommand{\figSeqUmbrella}{fig/fig_anno/umbrella}

    % Set color remapping (can brighten images this way)

    % Set image size
    \newcommand{\imgw}{0.49\linewidth} % 5-across figure
     % 5-across half-width figure
    %\newcommand{\imgh}{1in}
    
    % Command to draw an image with a different color map + crop as needed
    \newcommand{\imgRGB}[2][0px 0px 0px 0px]{\includegraphics[draft=\isdraft,width=\imgw,trim=#1,clip]{#2}}

    % ^^^ NOTE DRAFT COMMAND!
    % Uncomment to actually show the pictures
    % ^^^

    \newcommand{\zoomRGB}[4]{
        \begin{tikzpicture}[
    		image/.style={inner sep=0pt, outer sep=0pt},
    		collabel/.style={above=9pt, anchor=north, inner ysep=0pt, align=center}, % scale=0.8
    		rowlabel/.style={left=9pt, rotate=90, anchor=north, inner ysep=0pt, scale=0.8, align=center},
    		subcaption/.style={inner xsep=0.75mm, inner ysep=0.75mm, below right},
    		arrow/.style={-{Latex[length=2.5mm,width=4mm]}, line width=2mm},
    		spy using outlines={rectangle, size=1.25cm, magnification=3, connect spies, ultra thick, every spy on node/.append style={thick}},
    		style1/.style={cyan!90!black,thick},
    		style2/.style={orange!90!black},
    		style3/.style={blue!90!black},
    		style4/.style={green!90!black},
    		style5/.style={white},
    		style6/.style={black},
        ]
        
        \node [image] (#1) {\imgRGB[100px 0px 0px 0px]{#2}};
        \spy[style5] on ($(#1.center)-#3$) in node (crop-#1) [anchor=#4] at (#1.#4);
        
        \end{tikzpicture}
    }

    \scriptsize
    \begin{tabular}{c c c}
    
    % Legend.
    % Note: first column is rotated sequence title

    %%%%%%%%%%%%%%%%%%%%%%%%%
    % Sequence: Features

    % Labels
    &
    Input &
    Annotation
    \\ 
    
    \rotatebox{90}{\hspace{0.3cm} \seqBalloonNoticeBoard} &
    \imgRGB[45px 0px 0px 0px]{\figSeqBalloon/00000.png} &
    \imgRGB[45px 0px 0px 0px]{\figSeqBalloon/training_ 0.png} \\

    \rotatebox{90}{\hspace{0.5cm} \seqBalloonWall} &
    \imgRGB[45px 0px 0px 0px]{\figSeqBalloonw/00000.png} &
    \imgRGB[45px 0px 0px 0px]{\figSeqBalloonw/training_ 0.png}
    \\

    \rotatebox{90}{\hspace{0.4cm} \seqDynamicFace} &
    \imgRGB[45px 0px 0px 0px]{\figSeqDynamicFace/00000.png} &
    \imgRGB[45px 0px 0px 0px]{\figSeqDynamicFace/training_ 0.png}    
    \\

    \rotatebox{90}{\hspace{0.7cm} \seqJumping} &
    \imgRGB[45px 0px 0px 0px]{\figSeqJumping/00000.png} &
    \imgRGB[45px 0px 0px 0px]{\figSeqJumping/training_ 0.png}
    \\

    \rotatebox{90}{\hspace{0.6cm} \seqUmbrella} &
    \imgRGB[45px 0px 0px 0px]{\figSeqUmbrella/00000.png} &
    \imgRGB[45px 0px 0px 0px]{\figSeqUmbrella/training_ 0.png}   

    \end{tabular}

    \vspace{-0.25cm}
    \caption{
        \textbf{Manually annotated object masks.} We store annotation masks as grayscale images. The background is assigned as pixel value $0$, and foreground instances are each assigned a unique non-zero value.
    }
    \vspace{10cm}
    \label{fig:data annotate}
\end{figure}

}
\vfill

%%%%%%%%%%%%%%%%%%%%%%%%%%%%%%%%%%%%%
\clearpage
\section{NSFF Extra Scene}
Apart from \dataname, the NSFF~\cite{li2020neural} authors shared a \emph{kid-running} scene to help explain their method and as a test example in their code release. Along with the smartphone sequences in DyCheck~\cite{gao2022dynamic}, this is also a `true' monocular sequence captured with a single handheld camera. We demonstrate \titlename's decomposition result on this sequence to further demonstrate our semantic attention approach (\cref{fig:kid_running}).

%%%%%%%%%%%%%%%%%%%%%%%%%%%%%%%%%
%  KidRunning 
%%%%%%%%%%%%%%%%%%%%%%%%%%%%%%%%%

{   % Scope declared variables

\begin{figure*}[t]
    \centering
    %\setlength{\tabcolsep}{1pt}
    
    % Set figure images paths for sequences
    \newcommand{\figSeqKid}{fig/fig_kidrunning}

    % Set color remapping (can brighten images this way)

    % Set image size
    \newcommand{\imgw}{0.22\linewidth}
    %\newcommand{\imgh}{0.01\linewidth}
    
    % Command to draw an image with a different color map + crop as needed
    \newcommand{\imgRGB}[2][0px 0px 0px 0px]{\includegraphics[draft=\isdraft,width=\imgw,trim=#1,clip]{#2}}

    % ^^^ NOTE DRAFT COMMAND!
    % Uncomment to actually show the pictures
    % ^^^
    
    \newcommand{\zoomRGB}[4]{
        \begin{tikzpicture}[
    		image/.style={inner sep=0pt, outer sep=0pt},
    		collabel/.style={above=9pt, anchor=north, inner ysep=0pt, align=center}, % scale=0.8
    		rowlabel/.style={left=9pt, rotate=90, anchor=north, inner ysep=0pt, scale=0.8, align=center},
    		subcaption/.style={inner xsep=0.75mm, inner ysep=0.75mm, below right},
    		arrow/.style={-{Latex[length=2.5mm,width=4mm]}, line width=2mm},
    		spy using outlines={rectangle, size=1.25cm, magnification=3, connect spies, ultra thick, every spy on node/.append style={thick}},
    		style1/.style={cyan!90!black,thick},
    		style2/.style={orange!90!black},
    		style3/.style={blue!90!black},
    		style4/.style={green!90!black},
    		style5/.style={white},
    		style6/.style={black},
        ]
        
        \node [image] (#1) {\imgRGB{#2}};
        \spy[style5] on ($(#1.center)-#3$) in node (crop-#1) [anchor=#4] at (#1.#4);
        
        \end{tikzpicture}
    }
    
    \begin{tabular}{c c@{\hspace{0.2mm}} c@{\hspace{0.2mm}} c@{\hspace{0.2mm}} c@{\hspace{0.2mm}} c}
    
    % Legend.
    % Note: first column is rotated sequence title
    & 
    (a) Ground Truth &
    (b) RGB Rendering & 
    (c) Depth Rendering &
    (d) Decomposition  \\
    
     %%%%%%%%%%%%%%%%%%%%%%%%%
    % Sequence: DynamicFace-2
    \rotatebox{90}{\footnotesize \datasplitInput} % This centers the text

    &
    \imgRGB[45px 0px 90px 0px]{\figSeqKid/00043.png}
     &
    
     \imgRGB[45px 0px 90px 0px]{\figSeqKid/43_rgb.png}&
    
     \imgRGB[45px 0px 90px 0px]{\figSeqKid/43_depth.png} &
    
    \imgRGB[45px 0px 90px 0px]{\figSeqKid/43_cluster.png}

    \\[-1pt]

    %%%%%%%%%%%%%%%%%%%%%%%%%
    % Sequence: Balloon 1 (Notice Board)
    \rotatebox{90}{\footnotesize \datasplitTest} % This centers the text

    &
     \imgRGB[45px 0px 90px 0px]{\figSeqKid/00026.png} &
    
     \imgRGB[45px 0px 90px 0px]{\figSeqKid/26_rgb.png} &
    
     \imgRGB[45px 0px 90px 0px]{\figSeqKid/26_depth.png} &
    
     \imgRGB[45px 0px 90px 0px]{\figSeqKid/26_cluster.png} 

    \\[-1pt]

     %%%%%%%%%%%%%%%%%%%%%%%%%

    %%%%%%%%%%%%%%%%%%%%%%%%%
   
    %%%%%%%%%%%%%%%%%%%%%%%%%
    % Sequence: xxx

    % In general, we will pick a small set of sequences that show off key properties of our method.

    \end{tabular}

    \vspace{-0.25cm}
    \caption{
        \titlename's rendering and decomposition result on the \emph{kid-running} scene.
    }
    \label{fig:kid_running}
\end{figure*}

}

% Design choices
%\clearpage
\section{Design Choices}
\label{sec:designchoices}

\subsection{Underlying Dynamic NeRF Approach}

\paragraph{View synthesis and depth}
First, we evaluate whether RGB view synthesis performance is affected by adding more heads to the MLP. We find that it is not affected (\cref{tab:rgb_noharm}). \ddnerf's hyper-spacetime deformation has trouble reconstructing images on this dataset, producing distorted dynamic objects or failing to freeze time. 
% For scene geometry over time (depth), we produce similar results to NSFF (cf.~in our supplement).

In \cref{fig:viewsynthesis_rgbdepth}, we show qualitatively that \titlename does not degrade view synthesis or depth quality compared to NSFF~\cite{li2020neural}, while \ddnerf struggles with our data.

\paragraph{Why does \ddnerf struggle?} 
The main distinction is that \ddnerf is a deformation-based method while NSFF and \titlename are flow-based methods. For \ddnerf, the scene is reconstructed in a canonical space and deformed to render the results. \ddnerf struggles with larger motion in the scene---in the NVIDIA dataset, it is notably more difficult to find temporal correspondence within because frames are spatially far apart (unlike other monocular datasets created from one video camera only). Given only a monocular video to describe a scene with large camera motion \emph{and} large object motion, it appears difficult to faithfully reconstruct both the canonical space and the deformation. 
In comparison, \ddnerf produces good RGB reconstructions on the Nerfies~\cite{park2021nerfies} dataset because both the camera and scene motion are smaller than in the NVIDIA Dynamic Scene Dataset.

% View synthesis experiment
{
\setlength{\tabcolsep}{0.25em}
\begin{table}[tb]

    \centering
    
    \caption{
        \textbf{SAFF does not degrade image quality.} Adding semantics and attention on the same backbone produces the same image quality as NSFF~\cite{li2020neural}. Metrics: L is LPIPS ($[0,1]$, lower is better), S is SSIM ($[0,1]$, higher is better), P is PSNR ($[0,\infty]$, higher is better). \label{tab:rgb_noharm}
    }
    %\vspace{-0.25cm}
    
    \resizebox{1.0\linewidth}{!}{
    \begin{tabular}{l c c c c c c c c c}
    \toprule
    {} & \multicolumn{3}{c}{\datasplitInput} & \multicolumn{3}{c}{\datasplitCamZero} & \multicolumn{3}{c}{\datasplitTimeZero} \\
    %{} & LPIPS & SSIM & PSNR & LPIPS & SSIM & PSNR & LPIPS & SSIM & PSNR \\
    {} & L \tridown & S \triup & P \triup & L & S & P & L & S & P \\
    \midrule
    \ddnerf             & 0.115 & 0.790 & 23.91 & 0.228 & 0.565 & 18.04 & 0.344 & 0.309 & 13.85 \\
    NSFF w/o masks      & 0.070 & 0.805 & 23.92 &   0.100 & 0.762 & 21.68 &  0.302 & 0.386 & 14.92 \\
    \titlename (ours)   & 0.070 & 0.805 & 23.92 &   0.100 & 0.762 & 21.70 &  0.302 & 0.386 & 14.93 \\
    \bottomrule
    
    \end{tabular}
    }
    %\vspace{-0.5cm}
    
\end{table}
}

{
\begin{figure*}[t]
    \centering
    \setlength{\tabcolsep}{1pt}
    
    % Set figure images paths for sequences
    % \newcommand{\figSeqJumping}{fig/fig_foreground/jumping}
    \newcommand{\figSeqBalloon}{fig/fig_rgb/balloon}
    \newcommand{\figSeqBalloonw}{fig/fig_rgb/balloon2}
    \newcommand{\figSeqDynamicFace}{fig/fig_rgb/dynamicFace}
    \newcommand{\figSeqJumping}{fig/fig_rgb/jumping}
    \newcommand{\figSeqSkating}{fig/fig_rgb/skating}
    
    \newcommand{\figSeqTruck}{fig/fig_rgb/truck}
    \newcommand{\figSeqUmbrella}{fig/fig_rgb/umbrella}

    % Set color remapping (can brighten images this way)

    % Set image size
    \newcommand{\imgw}{0.24\linewidth} % 5-across figure
     % 5-across half-width figure

    % Command to draw an image with a different color map + crop as needed
    \newcommand{\imgRGB}[2][0px 0px 0px 0px]{\includegraphics[draft=\isdraft,width=\imgw,height=\imgh,trim=#1,clip]{#2}}

    % ^^^ NOTE DRAFT COMMAND!
    % Uncomment to actually show the pictures
    % ^^^

    \newcommand{\zoomRGB}[4]{
        \begin{tikzpicture}[
    		image/.style={inner sep=0pt, outer sep=0pt},
    		collabel/.style={above=9pt, anchor=north, inner ysep=0pt, align=center}, % scale=0.8
    		rowlabel/.style={left=9pt, rotate=90, anchor=north, inner ysep=0pt, scale=0.8, align=center},
    		subcaption/.style={inner xsep=0.75mm, inner ysep=0.75mm, below right},
    		arrow/.style={-{Latex[length=2.5mm,width=4mm]}, line width=2mm},
    		spy using outlines={rectangle, size=1.25cm, magnification=3, connect spies, ultra thick, every spy on node/.append style={thick}},
    		style1/.style={cyan!90!black,thick},
    		style2/.style={orange!90!black},
    		style3/.style={blue!90!black},
    		style4/.style={green!90!black},
    		style5/.style={white},
    		style6/.style={black},
        ]
        
        \node [image] (#1) {\imgRGB[45px 0px 0px 0px]{#2}};
        \spy[style5] on ($(#1.center)-#3$) in node (crop-#1) [anchor=#4] at (#1.#4);
        
        \end{tikzpicture}
    }

    \newcommand{\zoomRGBDDNeRF}[4]{
        \begin{tikzpicture}[
    		image/.style={inner sep=0pt, outer sep=0pt},
    		collabel/.style={above=9pt, anchor=north, inner ysep=0pt, align=center}, % scale=0.8
    		rowlabel/.style={left=9pt, rotate=90, anchor=north, inner ysep=0pt, scale=0.8, align=center},
    		subcaption/.style={inner xsep=0.75mm, inner ysep=0.75mm, below right},
    		arrow/.style={-{Latex[length=2.5mm,width=4mm]}, line width=2mm},
    		spy using outlines={rectangle, size=1.25cm, magnification=3, connect spies, ultra thick, every spy on node/.append style={thick}},
    		style1/.style={cyan!90!black,thick},
    		style2/.style={orange!90!black},
    		style3/.style={blue!90!black},
    		style4/.style={green!90!black},
    		style5/.style={white},
    		style6/.style={black},
        ]
        
        \node [image] (#1) {\imgRGB[40px 0px 0px 0px]{#2}};
        \spy[style5] on ($(#1.center)-#3$) in node (crop-#1) [anchor=#4] at (#1.#4);
        
        \end{tikzpicture}
    }

    \scriptsize
    \begin{tabular}{c c@{\hspace{0.2mm}} c@{\hspace{0.2mm}} c@{\hspace{0.2mm}} c@{\hspace{0.2mm}}  c}
    
    % Legend.
    % Note: first column is rotated sequence title

    %%%%%%%%%%%%%%%%%%%%%%%%%
    % Sequence: Features

    % Labels
    &
    GT &
    NSFF~\cite{li2020neural} &
    \ddnerf~\cite{wu2022ddnerf} & 
    \titlename (ours) &
    \\    

    % %%%%%%%%%%%%%%%%%%%%%%%
    % % Sequence Notice Board
    % % Images for RGB 
    % %
    % \rotatebox{90}{\hspace{0.3cm} \seqBalloonNoticeBoard} &
     
    % \zoomRGB{balloonnb-gt}{\figSeqBalloon/cam01_2.png}{(-0.9,0.6)}{south west} &

    % \zoomRGB{balloonnb-nsff}{\figSeqBalloon/45_rgb_NSFF.png}{(-0.9,0.6)}{south west} &
    
    % \zoomRGBDDNeRF{balloonnb-ddnerf}{\figSeqBalloon/regular_rgb_000021.png}{(-0.7,0.6)}{south west} &
    
    % \zoomRGB{balloonnb-saff}{\figSeqBalloon/45_rgb.png}{(-0.9,0.6)}{south west}
    % \\
    
    % % Images for depth
    % %
    % &
    % &
    % \zoomRGB{balloonnb-depth-nsff}{\figSeqBalloon/45_depth_NSFF.png}{(-0.9,0.6)}{south west} &

    % \zoomRGB{balloonnb-depth-ddnerf}{\figSeqBalloon/45_depth_d2nerf.png}{(-0.9,0.6)}{south west} &

    % \zoomRGB{balloonnb-depth-saff}{\figSeqBalloon/45_depth_saff.png}{(-0.9,0.6)}{south west}
    % \\

    %%%%%%%%%%%%%%%%%%%%%
    % % Sequence Balloon Wall
    % %
    % \rotatebox{90}{\hspace{0.45cm} \seqBalloonWall} &
    
    % \imgRGB[45px 0px 0px 0px]{\figSeqBalloonw/cam01_3.png} &

    % \imgRGB[45px 0px 0px 0px]{\figSeqBalloonw/41_rgb_NSFF.png} &
    
    % \imgRGB[40px 0px 0px 0px]{\figSeqBalloonw/regular_rgb_017.png} &
    
    % \imgRGB[45px 0px 0px 0px]{\figSeqBalloonw/41_rgb.png}
    % \\  

    %%%%%%%%%%%%%%%%%%
    % Sequence Dynamic Face
    %
    \rotatebox{90}{\hspace{0.35cm} \seqDynamicFace} &

    \zoomRGB{dynamicface-gt}{\figSeqDynamicFace/cam09.png}{(0,-0.2)}{south west} &

    \zoomRGB{dynamicface-nsff}{\figSeqDynamicFace/56_rgb_NSFF.png}{(0,-0.2)}{south west} &
    
    \zoomRGBDDNeRF{dynamicface-ddnerf}{\figSeqDynamicFace/regular_rgb_020.png}{(0.2,-0.2)}{south west} &
    
    \zoomRGB{dynamicface-saff}{\figSeqDynamicFace/56_rgb.png}{(0,-0.2)}{south west}
    \\  
    
    % Images for depth
    %
    &
    &
    \zoomRGB{dynamicface-depth-nsff}{\figSeqDynamicFace/56_depth_NSFF.png}{(-0.2,0.1)}{south west} &

    \zoomRGB{dynamicface-depth-ddnerf}{\figSeqDynamicFace/regular_depth_020.png}{(0.45,0.18)}{south west} &

    \zoomRGB{dynamicface-depth-saff}{\figSeqDynamicFace/56_depth.png}{(-0.2,0.1)}{south west}
    \\
    
    %%%%%%%%%%%%%%%%%%%%
    %% Sequence Umbrella
    %% Images for RGB
    %% %
    % \rotatebox{90}{\hspace{0.7cm} \seqJumping} &
    
    % \imgRGB[45px 0px 0px 0px]{\figSeqJumping/cam07.png} &

    % \imgRGB[45px 0px 0px 0px]{\figSeqJumping/54_rgb_NSFF.png} &
    
    % \imgRGB[40px 0px 0px 0px]{\figSeqJumping/regular_rgb_018.png} &
    
    % \imgRGB[45px 0px 0px 0px]{\figSeqJumping/54_rgb.png}
    % \\ 

    %%%%%%%%%%%%%%%%%%%
    % Sequence skating
    % Images for RGB
    %
    \rotatebox{90}{\hspace{0.7cm} \seqSkating} &
    
    \zoomRGB{skating-gt}{\figSeqSkating/cam08.png}{(1.1,0.3)}{south east} &

    \zoomRGB{skating-nsff}{\figSeqSkating/55_rgb_NSFF.png}{(1.1,0.3)}{south east} &
    
    \zoomRGBDDNeRF{skating-ddnerf}{\figSeqSkating/regular_rgb_019.png}{(1.3,0.3)}{south east} &
    
    \zoomRGB{skating-saff}{\figSeqSkating/55_rgb.png}{(1.1,0.3)}{south east}
    \\  

    % Images for depth
    %
    &
    &
    \zoomRGB{dynamicface-depth-nsff}{\figSeqSkating/55_depth_NSFF.png}{(-0.9,0.6)}{south west} &

    \zoomRGB{dynamicface-depth-ddnerf}{\figSeqSkating/regular_depth_019.png}{(-0.9,0.6)}{south west} &

    \zoomRGB{dynamicface-depth-saff}{\figSeqSkating/55_depth.png}{(-0.9,0.6)}{south west}
    \\

    %%%%%%%%%%%%%%%%%%%
    % Sequence Umbrella
    % Images for RGB
    %
    \rotatebox{90}{\hspace{0.6cm} \seqUmbrella} &
     
    \zoomRGB{umbrella-gt}{\figSeqUmbrella/cam10.png}{(0.8,-0.33)}{south east} &

    \zoomRGB{umbrella-nsff}{\figSeqUmbrella/57_rgb_NSFF.png}{(0.75,-0.3)}{south east} &
    
    \zoomRGBDDNeRF{umbrella-ddnerf}{\figSeqUmbrella/regular_rgb_021.png}{(0.75,-0.3)}{south east} &
    
    \zoomRGB{umbrella-saff}{\figSeqUmbrella/57_rgb.png}{(0.75,-0.3)}{south east}
    \\  

    % Images for depth
    %
    &
    &
    \zoomRGB{umbrella-depth-nsff}{\figSeqUmbrella/57_depth_NSFF.png}{(-0.9,0.6)}{south west} &

    \zoomRGB{umbrella-depth-ddnerf}{\figSeqUmbrella/regular_depth_021.png}{(-0.9,0.6)}{south west} &

    \zoomRGB{umbrella-depth-saff}{\figSeqUmbrella/57_depth.png}{(-0.9,0.6)}{south west}

    \end{tabular}

    \vspace{-0.25cm}
    \caption{
        \textbf{\titlename does not degrade novel spacetime view synthesis or depth quality.} \ddnerf struggles on the NVIDIA Dynamic Scene Dataset sequences because of the large motions between cameras.
    }
	
    \label{fig:viewsynthesis_rgbdepth}
    \vspace{-0.25cm}
\end{figure*}

}

%%%%%%%%%%%%%%%%%%%%%%%%%%%%%%%%%%%%%%%%%%%%%%%%%%%%%
\clearpage % new page
\subsection{3D vs.~2D Projected vs.~4D Spacetime Clustering}
\label{sec:spacetime4Dclustering}

In our saliency-aware clustering step, the elbow $k$-means method can take as input the per-pixel semantics features that have been sampled from 3D points in the volume (\textbf{in 3D}), or that have been rendered from the volume back to the 2D plane. Even though a volume is reconstructed, we find performance is somewhat worse when clustering in 3D than in projected 2D space (\cref{tab:spacetime4dclustering}; and in main paper). With respect to evaluation, it is difficult to collect ground truth segmented 3D data for dynamic real world scenes (none exist to our knowledge); this remains future work.

So, why might clustering in 3D lead to worse segmentations? Given monocular input from narrow baselines and dynamic scenes, the reconstruction can be imprecise with noisy geometry. This is in contrast to dynamic scenes captured with multi-camera setups or static scenes captured with wide baselines. 
% Thus, precise separation in 3D from monocular casually-captured videos is hard, leading to better clustering performance in volume-projected spacetime. 
%In the monocular input case with narrow baselines and dynamic scenes, it is challenging to precisely reconstruct geometries. 
As semantics and saliency use the same estimated geometry as radiance, clustering in the 3D volume introduces inaccuracy in the decomposition result, thus reducing the performance quantitatively and qualitatively. We visualize the volume as a point cloud from sampled 3D points in ~\cref{fig:fig3Dnoise}. Although the volume looks natural from the training view, erroneous regions are visible when the camera pose is far away from the training view, especially on the dynamic objects. 
%The incorrect geometry at those regions introduces noise into both semantics and saliency fields. }

Given direct clustering in 3D suffers from the narrow-baseline issue, we introduce another variant (\textbf{in 4D spacetime}) that also clusters upon a 3D position for each input pixel using the recovered volume density (from the estimated depth) and the timestep. While not the same as a volumetric clustering with some dense sampling, this sparse alternative is a reasonable computational compromise as our scenes contain opaque objects without participating media. We concatenate the spacetime coordinates with the semantic features for each pixel, then empirically adjust their relative weights to increase foreground segmentation performance.

In principle, this could exploit the underlying geometry to provide better edges or more instance awareness to the method. However, in practice, this does not reliably happen (\cref{tab:spacetime4dclustering}). 
Any error in alignment between the semantic information and the geometry causes the clustering to confuse elements, e.g., semantics for the same object at different depths over edge boundaries. As a consequence, semantically-different entities may not be correctly separated (\seqTruck), or are missing parts (\seqJumping, \cref{fig:spacetime4dclustering}). As such, we use only projected 2D semantic features as input to the clustering.

However, even though we use semantic-attention pyramids to increase the geometric resolution of the \semfeatnetwork features significantly, and even though volume integration increases these still (e.g., main paper, Figure 2), one might ask whether the optimization routine could also help further align the geometry and semantic features during volume integration. This brings us to the next subsection.

\begin{table}[t]
    \centering
    
    \caption{
        \textbf{3D volume clustering produces worse 2D segmentations than projected 2D clustering.} This is because precise localization of 3D geometry is difficult from monocular inputs for dynamic scenes. 4D spacetime clustering also produces worse foregrounds. Metric: Adjusted Rand Index ($[-1,1]$, higher is better). 
        \label{tab:spacetime4dclustering}
    }

    \vspace{-0.25cm}
    %\resizebox{\linewidth}{!}{
    \begin{tabular}{l r r r}
    
    \toprule
    {} & \datasplitInput & \datasplitCamZero & \datasplitTimeZero \\
    %{} & \multicolumn{3}{c}{ARI} \\
    
    \midrule
    
    \titlename (ours)                               &  \textbf{0.653}   &  \textbf{0.634}   & \textbf{0.625}  \\
    \hspace{0.2cm} in 3D                            &  0.594   &  0.578 &
    0.566 \\
    \hspace{0.2cm} in 4D spacetime                  &  0.482            &  0.464            & 0.452  \\
    
    \bottomrule 
    
    \end{tabular}
    %}
\end{table}
{
\begin{figure}[t]
    \centering
    \setlength{\tabcolsep}{1pt}
    
    % Set figure images paths for sequences
    % \newcommand{\figSeqJumping}{fig/fig_foreground/jumping}
    \newcommand{\figSeqBalloon}{fig/fig_anno/balloon}
    \newcommand{\figSeqBalloonw}{fig/fig_anno/balloon2}
    \newcommand{\figSeqDynamicFace}{fig/fig_anno/dynamicFace}
    \newcommand{\figSeqJumping}{fig/fig_anno/jumping}
    \newcommand{\figSeqSkating}{fig/fig_anno/skating}
    
    \newcommand{\figSeqTruck}{fig/fig_anno/truck}
    \newcommand{\figSeqUmbrella}{fig/fig_anno/umbrella}

    % Set color remapping (can brighten images this way)

    % Set image size
    \newcommand{\imgw}{0.49\linewidth} % 5-across figure
     % 5-across half-width figure
    %\newcommand{\imgh}{1in}
    
    % Command to draw an image with a different color map + crop as needed
    \newcommand{\imgRGB}[2][0px 0px 0px 0px]{\includegraphics[draft=\isdraft,width=\imgw,trim=#1,clip]{#2}}

    % ^^^ NOTE DRAFT COMMAND!
    % Uncomment to actually show the pictures
    % ^^^

    \newcommand{\zoomRGB}[4]{
        \begin{tikzpicture}[
    		image/.style={inner sep=0pt, outer sep=0pt},
    		collabel/.style={above=9pt, anchor=north, inner ysep=0pt, align=center}, % scale=0.8
    		rowlabel/.style={left=9pt, rotate=90, anchor=north, inner ysep=0pt, scale=0.8, align=center},
    		subcaption/.style={inner xsep=0.75mm, inner ysep=0.75mm, below right},
    		arrow/.style={-{Latex[length=2.5mm,width=4mm]}, line width=2mm},
    		spy using outlines={rectangle, size=1.25cm, magnification=3, connect spies, ultra thick, every spy on node/.append style={thick}},
    		style1/.style={cyan!90!black,thick},
    		style2/.style={orange!90!black},
    		style3/.style={blue!90!black},
    		style4/.style={green!90!black},
    		style5/.style={white},
    		style6/.style={black},
        ]
        
        \node [image] (#1) {\imgRGB[100px 0px 0px 0px]{#2}};
        \spy[style5] on ($(#1.center)-#3$) in node (crop-#1) [anchor=#4] at (#1.#4);
        
        \end{tikzpicture}
    }

    \scriptsize
    \begin{tabular}{c c}
    
    % Legend.
    % Note: first column is rotated sequence title

    %%%%%%%%%%%%%%%%%%%%%%%%%
    % Sequence: Features

    % Labels
    Training View &
    3D Side View
    \\ 
    \imgRGB[45px 50px 80px 50px]{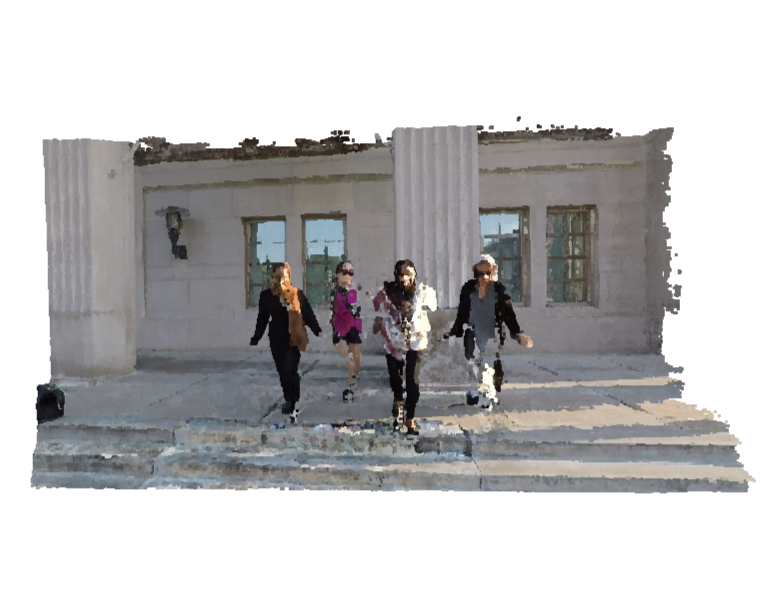} &
    \imgRGB[90px 50px 20px 50px]{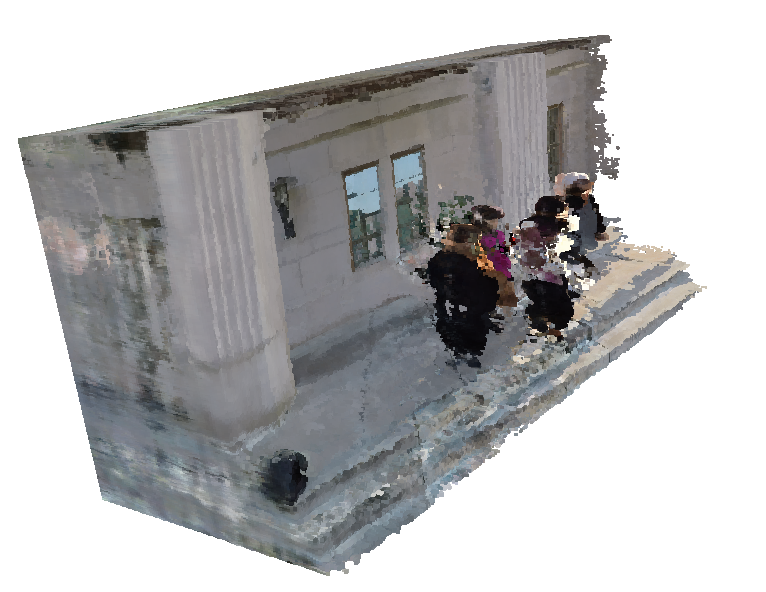}   

    \end{tabular}

    \vspace{-0.25cm}
    \caption{
        \textbf{3D samples.} Erroneous geometry reconstruction at regions invisible during training harms 3D clustering quality.
    }
    \label{fig:fig3Dnoise}
\end{figure}

}
{
\begin{figure}[t]
    \centering
        
    \setlength{\tabcolsep}{1pt}
    
    % Set figure images paths for sequences
    % \newcommand{\figSeqJumping}{fig/fig_foreground/jumping}
    \newcommand{\figSeqBalloon}{fig/fig_spacetime4Dclustering/balloon}
    \newcommand{\figSeqJumping}{fig/fig_spacetime4Dclustering/jumping}
    \newcommand{\figSeqTruck}{fig/fig_spacetime4Dclustering/truck}
    %\newcommand{\figSeqUmbrella}{fig/fig_anno/umbrella}

    % Set color remapping (can brighten images this way)

    % Set image size
    \newcommand{\imgw}{0.45\linewidth} % 5-across figure
     % 5-across half-width figure
    %\newcommand{\imgh}{1in}
    
    % Command to draw an image with a different color map + crop as needed
    \newcommand{\imgRGB}[2][0px 0px 0px 0px]{\includegraphics[draft=\isdraft,width=\imgw,trim=#1,clip]{#2}}

    % ^^^ NOTE DRAFT COMMAND!
    % Uncomment to actually show the pictures
    % ^^^

    \newcommand{\zoomRGB}[4]{
        \begin{tikzpicture}[
    		image/.style={inner sep=0pt, outer sep=0pt},
    		collabel/.style={above=9pt, anchor=north, inner ysep=0pt, align=center}, % scale=0.8
    		rowlabel/.style={left=9pt, rotate=90, anchor=north, inner ysep=0pt, scale=0.8, align=center},
    		subcaption/.style={inner xsep=0.75mm, inner ysep=0.75mm, below right},
    		arrow/.style={-{Latex[length=2.5mm,width=4mm]}, line width=2mm},
    		spy using outlines={rectangle, size=1.25cm, magnification=3, connect spies, ultra thick, every spy on node/.append style={thick}},
    		style1/.style={cyan!90!black,thick},
    		style2/.style={orange!90!black},
    		style3/.style={blue!90!black},
    		style4/.style={green!90!black},
    		style5/.style={white},
    		style6/.style={black},
        ]
        
        \node [image] (#1) {\imgRGB[100px 0px 0px 0px]{#2}};
        \spy[style5] on ($(#1.center)-#3$) in node (crop-#1) [anchor=#4] at (#1.#4);
        
        \end{tikzpicture}
    }

    \scriptsize
    \begin{tabular}{c c@{\hspace{0.2mm}} c@{\hspace{0.2mm}}   c}
    
    % Legend.
    % Note: first column is rotated sequence title

    %%%%%%%%%%%%%%%%%%%%%%%%%%%%%% 
    % Labels
    &
    \seqJumping &
    \seqTruck
    \\    

    %%%%%%%%%%%%%%%%%%%%%%%%%%%%%%
    % Input images
    %
    \rotatebox{90}{\hspace{0.8cm} Input} &

    \imgRGB[45px 0px 0px 0px]{\figSeqJumping/00009.png} &
    
    \imgRGB[45px 0px 0px 0px]{\figSeqTruck/00017.png} 
    \\

    %%%%%%%%%%%%%%%%%%%%%%%%%%%%%%
    % 3D clustering
    
    % Labels for pyramid preprocess
    \rotatebox{90}{\hspace{0.35cm} w/ 3D} &

    \imgRGB[45px 0px 0px 0px]{\figSeqJumping/9_3D.png} &
    
    \imgRGB[45px 0px 0px 0px]{\figSeqTruck/17_3D.png} 
    \\

    %%%%%%%%%%%%%%%%%%%%%%%%%%%%%%
    % Spacetime clustering
    
    % Labels for pyramid preprocess
    \rotatebox{90}{\hspace{0.35cm} w/ spacetime} &

    \imgRGB[45px 0px 0px 0px]{\figSeqJumping/9_4D.png} &
    
    \imgRGB[45px 0px 0px 0px]{\figSeqTruck/17_4D.png} 
    \\

    %%%%%%%%%%%%%%%%%%%%%%%%%%%%%%
    % Projected 2D clustering
    \rotatebox{90}{\hspace{0.9cm} Ours} &

    \imgRGB[45px 0px 0px 0px]{\figSeqJumping/9.png} &
    
    \imgRGB[45px 0px 0px 0px]{\figSeqTruck/17.png} 
    \\

    \end{tabular}

    \vspace{-0.25cm}
    \caption{
        Clustering upon sampled 3D volume features or adding 4D spacetime features produces worse foregrounds qualitatively than just projected 2D feature clustering. This is because the narrow-baseline monocular input sometimes leads to noisy geometry estimation, and because the semantic edges must conform to the same geometry of the scene as the radiance. In 4D spacetime clustering, some clusters are confused or unnecessarily merged.
    }
	
    \label{fig:spacetime4dclustering}
\end{figure}

}

%%%%%%%%%%%%%%%%%%%%%%%%%%%%%%%%%%%%%%%%%%%%%
\clearpage % new page
\subsection{Decaying Semantics and Attention}
\label{sec:decaysemantics}

One way to improve the alignment of depth edges and semantic and attention features is through decaying their reconstruction loss through training. This decay happens to the depth and optical flow priors, and for those channels of information the decay provides freedom to the optimization to refine the spacetime density once initialized with respect to the self-consistent multi-view and scene flow constraints. Intuitively, decaying the semantics and attention reconstructions would also provide more freedom to further optimize the spacetime density to minimize the self-consistent multi-view and scene flow constraints when the semantics disagreed. 

However, in the main paper, we describe that semantics and attention are not priors---there is no self-consistency for semantics to constrain their values, thus, after decay the optimization is free for them to vary inconsistently and so for their reprojection to lose useful meaning. This could have unwanted consequences.

To investigate this design choice, we implement variant \textbf{w/ decay} in which we use the same decaying mechanism as depth and optical flow on $\lossSAFFsem$ and $\lossSAFFatt$. 
We also decay $\lossSAFFsemproj$ and $\lossSAFFattproj$, because the semantics are not necessarily consistent with the spacetime geometry.
% \jt{Find argument for why we also decay scene flow losses.}

% \jt{Yiqing, why do we decay the semantic flow loss? We want to keep that. We only want to decay the reconstruction loss. NSFF doesn't decay the flow losses.}
% \YL{argument(one sure side-effect): decayed semantics and attention fields are not exactly "correct"; in this case not decaying their flow may erroneously twist them to do their best to match the flow constrains but degrade to meaningless values }

Qualitatively, adding decay does better align the semantics and attention fields with the geometry, e.g., in \seqSkating, the space between skater's legs are better segmented; however, the clustering performance degrades all over the image (\cref{fig:decay}), e.g., in \seqSkating, now including a sconce and unwanted floor details (zoom in). This is also reflected quantitatively (\cref{tab:decay}).

{
\begin{figure}[t]
    \centering
    \setlength{\tabcolsep}{1pt}
    
    % Set figure images paths for sequences
    % \newcommand{\figSeqJumping}{fig/fig_foreground/jumping}
    %\newcommand{\figSeqBalloon}{fig/fig_anno/balloon}
    \newcommand{\figSeqBalloonw}{fig/fig_decay/balloon2}
    \newcommand{\figSeqSkating}{fig/fig_decay/skating}
    %\newcommand{\figSeqPlayground}{fig/fig_anno/playground}
    %\newcommand{\figSeqTruck}{fig/fig_anno/truck}
    %\newcommand{\figSeqUmbrella}{fig/fig_anno/umbrella}

    % Set color remapping (can brighten images this way)

    % Set image size
    \newcommand{\imgw}{0.45\linewidth} % 5-across figure
     % 5-across half-width figure
    %\newcommand{\imgh}{1in}
    
    % Command to draw an image with a different color map + crop as needed
    \newcommand{\imgRGB}[2][0px 0px 0px 0px]{\includegraphics[draft=\isdraft,width=\imgw,trim=#1,clip]{#2}}

    % ^^^ NOTE DRAFT COMMAND!
    % Uncomment to actually show the pictures
    % ^^^

    \newcommand{\zoomRGB}[4]{
        \begin{tikzpicture}[
    		image/.style={inner sep=0pt, outer sep=0pt},
    		collabel/.style={above=9pt, anchor=north, inner ysep=0pt, align=center}, % scale=0.8
    		rowlabel/.style={left=9pt, rotate=90, anchor=north, inner ysep=0pt, scale=0.8, align=center},
    		subcaption/.style={inner xsep=0.75mm, inner ysep=0.75mm, below right},
    		arrow/.style={-{Latex[length=2.5mm,width=4mm]}, line width=2mm},
    		spy using outlines={rectangle, size=1.25cm, magnification=3, connect spies, ultra thick, every spy on node/.append style={thick}},
    		style1/.style={cyan!90!black,thick},
    		style2/.style={orange!90!black},
    		style3/.style={blue!90!black},
    		style4/.style={green!90!black},
    		style5/.style={white},
    		style6/.style={black},
        ]
        
        \node [image] (#1) {\imgRGB[45px 0px 0px 0px]{#2}};
        \spy[style5] on ($(#1.center)-#3$) in node (crop-#1) [anchor=#4] at (#1.#4);
        
        \end{tikzpicture}
    }

    \scriptsize
    \begin{tabular}{c c@{\hspace{0.2mm}} c@{\hspace{0.2mm}} c}
    
    % Legend.
    % Note: first column is rotated sequence title

    &
    (a) Balloon Wall &
    (b) Skating
    \\
    %%%%%%%%%%%%%%%%%%%%%%%%%
    % Sequence: Features

    % Labels
    %&
    %Balloon1-2 &
    %Balloon2-2 &
    %DynamicFace-2 & 
    %Jumping &
    %Umbrella
    %\\    

    \rotatebox{90}{Input} &

    \imgRGB[45px 0px 0px 0px]{\figSeqBalloonw/00015.png} &

    \imgRGB[45px 0px 0px 0px]{\figSeqSkating/00009.png} 
    \\

    % Images for pyramid preprocess
    %
    \rotatebox{90}{Ours+Decay} &
    
    \zoomRGB{balloon-decay}{\figSeqBalloonw/15_1.png}{(-0.2,0.4)}{north west} &

    \zoomRGB{skater-decay}{\figSeqSkating/9_1.png}{(0.9,-0.5)}{north east}
    \\

    %%%%%%%%%%%%%%%%%%%%%%%%%%%%%%
    % Sequence: Pyramid preprocess
    
    % Labels for pyramid preprocess
    \rotatebox{90}{Ours} &
     
    \zoomRGB{balloon-ours}{\figSeqBalloonw/15.png}{(-0.2,0.4)}{north west} &

    \zoomRGB{skater-ours}{\figSeqSkating/9.png}{(0.9,-0.5)}{north east}
    \\

    \end{tabular}

    \vspace{-0.25cm}
    \caption{
        \textbf{Decaying semantics and attention leads to missing objects and unwanted objects.} With no self-consistent constraint, the optimization is more free to adjust the meaning of regions. While this can increase edge detail, it creates worse overall results.
    }
	
    \label{fig:decay}
    \vspace{9cm}
\end{figure}

}
\begin{table}[t]
    \centering
    
    \caption{
        \textbf{Decaying semantic and attention information produces overall foregrounds.} While geometric alignment improves, semantic meaning also shifts, which harms the ability of the model to correctly identify salient objects. Metric: Adjusted Rand Index ($[-1,1]$, higher is better). 
        \label{tab:decay}
        }

    \vspace{-0.25cm}
    %\resizebox{\linewidth}{!}{
    \begin{tabular}{l r r r}
    
    \toprule
    {} & \datasplitInput & \datasplitCamZero & \datasplitTimeZero \\
    %{} & \multicolumn{3}{c}{ARI} \\
    
    \midrule
    
    \titlename (ours)           &  \textbf{0.653}   &  \textbf{0.634}   & \textbf{0.625}  \\
    \hspace{0.2cm} w/ decay     &  0.592            &  0.568            & 0.554  \\
    
    \bottomrule 
    
    \end{tabular}
    %}
\end{table}

\vfill

%%%%%%%%%%%%%%%%%%%%%%%%%%%%%%%%%
\clearpage % new page
\subsection{Pyramid Construction}
\label{sec:pyramidconstruction}

Figure~\ref{fig:pyramidconstruction} provides a diagrammatic example for how we construct our feature pyramids. We also provide algorithm pseudocode (\cref{alg:pyr_final}).

As mentioned in the main paper, given the pyramid layers, we begin conceptually from a weighted sum of three layers for semantics using $\lambdaSAFFsem\! =\! \{\nicefrac{1}{3},\nicefrac{1}{3},\nicefrac{1}{3} \}$ and with coarsest whole-image attention with $\lambdaSAFFatt\! =\! \{1,0,0\}$. This already gives quantitatively better decomposition performance than without using a pyramid (\textbf{w/o pyr}; \cref{tab:pyramiddecompose}). However, the optimized semantic field does not correspond as well to scene geometry and is more influenced by error in the coarsest layer semantics and attention than our approach. For instance, the human is not identified as salient in \seqBalloonNoticeBoard (\cref{fig:pyramid_compare}). Additionally, as the finer layer sliding windows do not typically contain the object of interest in boundary regions, the extracted features are incorrect. This causes unwanted clusters to appear around image edges, e.g., the gray cluster in the top right corner in \seqUmbrella (\cref{fig:pyramid_compare}).

To increase semantic and attention resolution, we increase $\lambdaSAFFsem\!$'s dependency on finer layers to $\! \{\nicefrac{4}{9},\nicefrac{4}{9},\nicefrac{1}{9} \}$. To deal with the boundary issues, we decrease the weight of fine layers towards the boundary back to $\! \{\nicefrac{1}{3},\nicefrac{1}{3},\nicefrac{1}{3} \}$. The image boundary problem is resolved in \seqUmbrella (\cref{fig:pyramid_compare}). However, there is still a mismatch between the fidelity of the semantics and saliency (the head disappears in \seqDynamicFace), which is also reflected quantitatively (\cref{tab:pyramiddecompose}).

Thus, we use the same weight proportions and boundary reduction for both semantics and attention. This strikes a balance between correct edges from fine layers and whole object features from coarse layers, and mitigates the feature noise around image boundaries. This yields the best overall results both qualitatively on balance (\cref{fig:pyramid_compare}) and quantitatively (\cref{tab:pyramiddecompose}).

% Force a new column so that the table is on the right.
\newpage

% Figma source:
% https://www.figma.com/file/7K2MNU1EsIEMZ1Or0IP5jK/CVPR-2023---Semantic-Attention-Flow-Fields?type=design&node-id=0-1&mode=design&t=BDgEcSafjDzIa1Ik-0

\begin{figure}[t]
    \includegraphics[width=\linewidth]{}
    \caption{\textbf{Pyramid construction example.} This attempts to balance feature quality with computational cost by aggregating overlapping feature extraction blocks from different image resolutions.}
    \label{fig:pyramidconstruction}
\end{figure}
\begin{table}[t]
    \centering
    
    \caption{
        \textbf{Pyramid weighting choice.} Even though in our final algorithm the coarse layer has smaller weight, it balances high resolution edges from fine layers and whole object features from coarse layers while reducing geometry conflicts, and mitigate the feature noise around edges.  \\
        % Dataset: \dataname. 
        Metric: Adjusted Rand Index ($[-1,1]$, higher is better). 
        \label{tab:pyramiddecompose}
        }

    \vspace{-0.25cm}
    \resizebox{\linewidth}{!}{
    \begin{tabular}{l r r r}
    
    \toprule
    {} & \datasplitInput & \datasplitCamZero & \datasplitTimeZero \\
    %{} & \multicolumn{3}{c}{ARI} \\
    
    \midrule
    SAFF  \\
    \hspace{0.2cm} w/o pyr $\hat{\semfeat},\hat{\attfeat}$  &  0.545            &  0.532            & 0.521  \\
    \midrule
    \titlename (ours)                               &  \textbf{0.653}   &  \textbf{0.634}   & \textbf{0.625}  \\
    \hspace{0.2cm} w/ pyr $\lambdaSAFFatt = \{1,0,0\}$    &  0.620            &  0.598            & 0.592  \\
    \hspace{0.2cm} w/ pyr $\lambdaSAFFatt = \{1,0,0\},$    &   \multirow{2}{*}{0.631}  & \multirow{2}{*}{0.612} & \multirow{2}{*}{0.601}\\
    \hspace{0.2cm}        $\lambdaSAFFsem\! =\! \{\nicefrac{1}{3},\nicefrac{1}{3},\nicefrac{1}{3} \}$ &     ~        &  ~   & ~ \\
    \bottomrule 
    
    \end{tabular}
    }
\end{table}

{
\begin{figure*}[b]
    \centering
    \setlength{\tabcolsep}{1pt}
    
    % Set figure images paths for sequences
    % \newcommand{\figSeqJumping}{fig/fig_foreground/jumping}
    \newcommand{\figSeqBalloon}{fig/fig_pyramid/balloon}
    \newcommand{\figSeqDynamicFace}{fig/fig_pyramid/dynamicFace}
    \newcommand{\figSeqUmbrella}{fig/fig_pyramid/umbrella}

    % Set color remapping (can brighten images this way)

    % Set image size
    \newcommand{\imgw}{0.19\linewidth} % 5-across figure
     % 5-across half-width figure
    %\newcommand{\imgh}{1in}
    
    % Command to draw an image with a different color map + crop as needed
    \newcommand{\imgRGB}[2][0px 0px 0px 0px]{\includegraphics[draft=\isdraft,width=\imgw,trim=#1,clip]{#2}}

    % ^^^ NOTE DRAFT COMMAND!
    % Uncomment to actually show the pictures
    % ^^^

    \newcommand{\zoomRGB}[4]{
        \begin{tikzpicture}[
    		image/.style={inner sep=0pt, outer sep=0pt},
    		collabel/.style={above=9pt, anchor=north, inner ysep=0pt, align=center}, % scale=0.8
    		rowlabel/.style={left=9pt, rotate=90, anchor=north, inner ysep=0pt, scale=0.8, align=center},
    		subcaption/.style={inner xsep=0.75mm, inner ysep=0.75mm, below right},
    		arrow/.style={-{Latex[length=2.5mm,width=4mm]}, line width=2mm},
    		spy using outlines={rectangle, size=1.25cm, magnification=3, connect spies, ultra thick, every spy on node/.append style={thick}},
    		style1/.style={cyan!90!black,thick},
    		style2/.style={orange!90!black},
    		style3/.style={blue!90!black},
    		style4/.style={green!90!black},
    		style5/.style={white},
    		style6/.style={black},
        ]
        
        \node [image] (#1) {\imgRGB[100px 0px 0px 0px]{#2}};
        \spy[style5] on ($(#1.center)-#3$) in node (crop-#1) [anchor=#4] at (#1.#4);
        
        \end{tikzpicture}
    }

    \scriptsize
    \begin{tabular}{c c@{\hspace{0.2mm}} c@{\hspace{0.2mm}} c@{\hspace{0.2mm}} c@{\hspace{0.2mm}} c@{\hspace{0.2mm}} c}
    
    % Legend.
    % Note: first column is rotated sequence title
    
    & 
    Input & 
    w/o pyr & 
    Balanced $\lambdaSAFFsem$ + Global $\lambdaSAFFatt$ & 
    Weighted $\lambdaSAFFsem$ + Global $\lambdaSAFFatt$ & 
    Ours (Weighted $\lambdaSAFFsem$ + Weighted $\lambdaSAFFatt$) 
    \\

    %&
    %(a) Balloon NBoard &
    %(b) Umbrella
    %\\
    %%%%%%%%%%%%%%%%%%%%%%%%%
    % Sequence: Features

    % Labels
    %&
    %Balloon1-2 &
    %Balloon2-2 &
    %DynamicFace-2 & 
    %Jumping &
    %Umbrella
    %\\    

    \rotatebox{90}{\hspace{0.1cm} \seqBalloonNoticeBoard} &
     
    % \imgRGB[45px 0px 0px 0px]{\figSeqTwoDim/ezgif-frame-001.jpeg} &
    \imgRGB[45px 0px 0px 0px]{\figSeqBalloon/00006.png} &
    \imgRGB[45px 0px 0px 0px]{\figSeqBalloon/6.png} &
     \imgRGB[45px 0px 0px 0px]{\figSeqBalloon/6_0.png} &
     \imgRGB[45px 0px 0px 0px]{\figSeqBalloon/6_1.png} &
     \imgRGB[45px 0px 0px 0px]{\figSeqBalloon/6_ours.png} &

    %\imgRGB[100px 0px 0px 0px]{\figSeqVolume/ezgif-frame-001-render.jpeg} &
    %\imgRGB[45px 0px 0px 0px]{\figSeqBalloonw/00000.png} &

    %\imgAtt[34px 0px 0px 0px]{\figSeqTwoDim/ezgif-frame-001-sal.png} &    
    %\imgRGB[45px 0px 0px 0px]{\figSeqDynamicFace/00015.png} &
    
    % \imgAtt[100px 0px 0px 0px]{\figSeqVolume/0_sal.png} 
    %\imgRGB[45px 0px 0px 0px]{\figSeqJumping/00023.png} &
    
    % \imgAtt[100px 0px 0px 0px]{\figSeqVolume/0_sal.png} 
    %\imgRGB[45px 0px 0px 0px]{\figSeqUmbrella/00007.png} &
    \\

    % Images for pyramid preprocess
    %
    \rotatebox{90}{\hspace{0.4cm} \seqUmbrella} &
     
    % \imgRGB[45px 0px 0px 0px]{\figSeqTwoDim/ezgif-frame-001.jpeg} &
    \imgRGB[45px 0px 0px 0px]{\figSeqUmbrella/00019.png} &

    %\imgRGB[100px 0px 0px 0px]{\figSeqVolume/ezgif-frame-001-render.jpeg} &
    %\imgRGB[45px 0px 0px 0px]{\figSeqBalloonw/00000.png} &

    %\imgAtt[34px 0px 0px 0px]{\figSeqTwoDim/ezgif-frame-001-sal.png} &    
    %\imgRGB[45px 0px 0px 0px]{\figSeqDynamicFace/15_raw.png} &
    
    % \imgAtt[100px 0px 0px 0px]{\figSeqVolume/0_sal.png} 
    %\imgRGB[45px 0px 0px 0px]{\figSeqJumping/23_raw.png} &
    
    % \imgAtt[100px 0px 0px 0px]{\figSeqVolume/0_sal.png} 
    \imgRGB[45px 0px 0px 0px]{\figSeqUmbrella/19.png} &
    \imgRGB[45px 0px 0px 0px]{\figSeqUmbrella/19_0.png} &
    \imgRGB[45px 0px 0px 0px]{\figSeqUmbrella/19_1.png} &
    \imgRGB[45px 0px 0px 0px]{\figSeqUmbrella/19_ours.png} &
    
    \\
    
     %%%%%%%%%%%%%%%%%%%%%%%%%%%%%%
    % Sequence: Pyramid preprocess
    
    % Labels for pyramid preprocess
    \rotatebox{90}{\hspace{0.2cm} \seqDynamicFace} &
     
    % \imgRGB[45px 0px 0px 0px]{\figSeqTwoDim/ezgif-frame-001.jpeg} &
    \imgRGB[45px 0px 0px 0px]{\figSeqDynamicFace/00004.png} &

    %\imgRGB[100px 0px 0px 0px]{\figSeqVolume/ezgif-frame-001-render.jpeg} &
    %\imgRGB[45px 0px 0px 0px]{\figSeqBalloonw/training_ 0.png} &

    %\imgAtt[34px 0px 0px 0px]{\figSeqTwoDim/ezgif-frame-001-sal.png} &    
    %\imgRGB[45px 0px 0px 0px]{\figSeqDynamicFace/15.png} &
    
    % \imgAtt[100px 0px 0px 0px]{\figSeqVolume/0_sal.png} 
    %\imgRGB[45px 0px 0px 0px]{\figSeqJumping/23.png} &
    
    % \imgAtt[100px 0px 0px 0px]{\figSeqVolume/0_sal.png} 
    
    \imgRGB[45px 0px 0px 0px]{\figSeqDynamicFace/4.png} &
    \imgRGB[45px 0px 0px 0px]{\figSeqDynamicFace/4_0.png} &
    \imgRGB[45px 0px 0px 0px]{\figSeqDynamicFace/4_1.png} &
    \imgRGB[45px 0px 0px 0px]{\figSeqDynamicFace/4_ours.png} &
    \\

    \end{tabular}

    \vspace{-0.25cm}
    \caption{
        \textbf{Pyramid construction varies final output quality after clustering.} Without the pyramid, key objects are missing or undersegmented. Our approach captures the objects with fewest errors compared to the variants.
        %Each approach uses our saliency-aware clustering \cref{alg:cluster}.
        \\
        Balanced $\lambdaSAFFsem$ + Global $\lambdaSAFFatt$: $\lambdaSAFFsem\! =\! \{\nicefrac{1}{3},\nicefrac{1}{3},\nicefrac{1}{3} \}$ with $\lambdaSAFFatt\! =\! \{1,0,0\}$
        \\
        Weighted $\lambdaSAFFsem$ + Global $\lambdaSAFFatt$: semantic attention pyramid
        %\cref{alg:pyr_final} 
        with $\lambdaSAFFatt\! =\! \{1,0,0\}$
        \\
        Ours (Weighted $\lambdaSAFFsem$ + Weighted $\lambdaSAFFatt$): Our semantic attention pyramid 
        %\cref{alg:pyr_final}.
    }
	
    \label{fig:pyramid_compare}
\end{figure*}
}

\begin{algorithm*}[t]
    \caption{\textbf{Pyramid Construction Algorithm (Example).} Given an RGB image $I$ of size ($H \times W \times 3$) and a $D$-dimensional feature extractor $E : (A \times B \times 3) \mapsto (\nicefrac{A}{4} \times \nicefrac{B}{4} \times D)$, produce a processed feature map for the input image.}
    \label{alg:pyr_final}
    \begin{algorithmic}
        \Require $I \in R^{H \times W \times 3}$,  $E \gets dino\_vit8$, $H$, $W$, $D$
        \State $level0 \gets I$
        \State $level1 \gets \textsc{downsample}(I, 480, 256)$ \Comment{Downsample image to 480 $
        \times$ 256.}
        \State $level2 \gets \textsc{downsample}(I, 240, 128)$
        \State $all\_patches\_in\_imagespace \gets []$
        \For{$level \in [level0, level1, level2]$}
        \State $x \gets 0$
        \While{$x + 240 \leq W$}
        \State $y \gets 0$
        \While{$y + 128 \leq H$}
        \State $patch \gets level[y:y+128,x:x+240,:]$
        \State $feature\_patch \gets \textsc{upsample}(E(patch), 240, 128)$
        \State $patch\_in\_imagespace \gets \textsc{new\_null\_array}(H, W, D)$  \Comment{To hold features in their input image location.}
        \State $patch\_in\_imagespace[y:y+128,x:x+240,:] \gets feature\_patch$
        \State $all\_patches\_in\_imagespace.\textsc{append}(patch\_in\_imagespace)$
        \State $y \gets y + 64$
        \EndWhile
        \State $x \gets x + 64$
        \EndWhile
        \EndFor
        \State $output\_full \gets \textsc{non\_null\_average}(all\_patches\_in\_imagespace)$ \Comment{Element-wise average of non-null values.}
        \State $output \gets \textsc{pca}(output\_full, 64)$
        
    \end{algorithmic}
\end{algorithm*}

%Practically, we use \cref{alg:pyr_final} to compute the pyramid.

%\jt{Write condition names in Figure in this paragraph.}

%%%%%%%%%%%%%%%%%%%%%%%%%%%%%%%%%%%%%
% Implementation details
\clearpage
\section{Implementation Details}
\label{sec:implementation}

\paragraph{Semantics and Attention}

Following Amir \etal~\cite{amir2021deep}, for semantics we extract the 384-dim.~`key' facet from the \nth{11} layer of \semfeatnetwork, and for saliency we extract the 1-dim.~`attention' facet from the \nth{11} layer.
For the pyramid, we use three levels. The coarsest level 0 is downsampled to $240\times 128$. The finest level 2 is the input RGB size, with the mid level 1's size set between the two. For each level, we use \semfeatnetwork as a sliding window of size $240\times 128$ to extract a (8$\times$8 patch; stride 4) $60\times 32$ feature map (i.e., level 0 has only one window position). For fast computation, we set window stride to 64. Once extracted, we upsample and place each feature map within level 2's frame. Then, for each pixel, we mean average all features from all windows that intersected it.
% 's window size is $480\times 256$, while top level's window size is $240\times 128$. For each level, we select the stride to be half of the window size. For each window, we interpolate the content to be $240\times 128$, extract \semfeatnetwork features, interpolate the feature back to original window size, then mean average the features across windows that intersect each pixel. 
%
Finally, to fit within GPU VRAM, we perform PCA on all images' normalized extracted pyramid $\hat{\semfeat},\hat{\attfeat}$ features and keep the most important 64 dimensions. 
% Empirically, this does not hurt performance because each video's content only comes from some limited semantic space.

\paragraph{Clustering}
Any clustering method has hyperparameters (or thresholds) for it to make decisions about cluster assignment. We use the same hyperparameters for all sequences.

We use the GPU via Faiss~\cite{johnson2019billion}. Again to fit within GPU VRAM, we uniformly sample every fifth point for elbow-$k$ finding, then propagate cluster assignment to all points given $k$. We set the elbow-$k$ threshold to 0.975 and the max cluster number to 25, with 10 trials per $k$. We cluster on direction and so normalize each pixel's vector.

\paragraph{Object extraction}
To extract an object from the volume, we sample 3D points along each input ray, then compare their semantics to to existing projected 2D semantic cluster centroids. We assign each 3D point to its closest centroid. Then, we set non-salient cluster label points to have zero density.

% For each input image ray's volume point sample ($W\!\!\times\!\!H\times\!\!\#samples$), we query all fields, then assign each 3D point a cluster label given its feature and fitted centroids 
% \jt{semantic feature? do we do this by matching to the cluster centroids via cosine similarity?}. 
% We simply set non-salient cluster label points to have zero volume density. Then, we can render the extracted object at novel space-time views.
% % Post-processing: given rendered blending map, set map with value $<0.1$ locations to be black in color image
% On the rendered 2D color/depth image, we set all pixels that are assigned background label to be black/0.

\paragraph{Post process}
All quantitative results are \emph{without} this unless stated; only the main paper Table 3 line includes this. 
%As we want salient objects, we morphologically open and close (3$\times$3) projected clusters and then merge remaining small clusters ($<\!\!\!0.01\times\!$ image area) into their nearest neighbors.
As appearance and geometry information is embedded in the volume, we want to refine the decomposition results by constraining them to align with rendered RGB and depth images. Specifically, we apply a CRF~\cite{NIPS2011_beda24c1} with a pairwise Gaussian unary potential ($\theta_{\gamma}$=$3$, $w$=$15$), a pairwise bilateral RGB potential ($\theta_{\gamma}$=$40$, $\theta_{\beta}$=$13$, $w$=$10$), and a pairwise bilateral depth potential ($\theta_{\gamma}$=$40$, $\theta_{\beta}$=$13$, $w$=$20$).
Applying a CRF is similar to Amir et al.~\cite{amir2021deep} on \semfeatnetwork in 2D, but our spacetime volume-integrated geometry provides a much stronger constraint on where the true edge is over time.
% We do not refine edges beyond this (cf.~\cite{amir2021deep}). 
The contribution of post processing is showed in \cref{fig:postprocessed} qualitatively. We see that small unimportant regions are removed, while still maintaining thin features and fine details. This trade-off is an application-level decision.
% , merge semantic clusters with more than $x$ unconnected islands, and 
% 540 x 288 

{
\begin{figure}[t]
    \centering
    \setlength{\tabcolsep}{1pt}
    
    % Set figure images paths for sequences
    % \newcommand{\figSeqJumping}{fig/fig_foreground/jumping}
    %\newcommand{\figSeqBalloon}{fig/fig_anno/balloon}
    %\newcommand{\figSeqBalloonw}{fig/fig_anno/balloon2}
    \newcommand{\figSeqDynamicFace}{fig/fig_post/dynamicFace}
    \newcommand{\figSeqJumping}{fig/fig_post/jumping}
    %\newcommand{\figSeqSkating}{fig/fig_anno/skating}
    %\newcommand{\figSeqPlayground}{fig/fig_anno/playground}
    %\newcommand{\figSeqTruck}{fig/fig_anno/truck}
    %\newcommand{\figSeqUmbrella}{fig/fig_anno/umbrella}

    % Set color remapping (can brighten images this way)

    % Set image size
    \newcommand{\imgw}{0.47\linewidth} % 5-across figure
     % 5-across half-width figure
    %\newcommand{\imgh}{1in}
    
    % Command to draw an image with a different color map + crop as needed
    \newcommand{\imgRGB}[2][0px 0px 0px 0px]{\includegraphics[draft=\isdraft,width=\imgw,trim=#1,clip]{#2}}

    % ^^^ NOTE DRAFT COMMAND!
    % Uncomment to actually show the pictures
    % ^^^

    \newcommand{\zoomRGB}[4]{
        \begin{tikzpicture}[
    		image/.style={inner sep=0pt, outer sep=0pt},
    		collabel/.style={above=9pt, anchor=north, inner ysep=0pt, align=center}, % scale=0.8
    		rowlabel/.style={left=9pt, rotate=90, anchor=north, inner ysep=0pt, scale=0.8, align=center},
    		subcaption/.style={inner xsep=0.75mm, inner ysep=0.75mm, below right},
    		arrow/.style={-{Latex[length=2.5mm,width=4mm]}, line width=2mm},
    		spy using outlines={rectangle, size=1.25cm, magnification=3, connect spies, ultra thick, every spy on node/.append style={thick}},
    		style1/.style={cyan!90!black,thick},
    		style2/.style={orange!90!black},
    		style3/.style={blue!90!black},
    		style4/.style={green!90!black},
    		style5/.style={white},
    		style6/.style={black},
        ]
        
        \node [image] (#1) {\imgRGB[100px 0px 0px 0px]{#2}};
        \spy[style5] on ($(#1.center)-#3$) in node (crop-#1) [anchor=#4] at (#1.#4);
        
        \end{tikzpicture}
    }

    \scriptsize
    \begin{tabular}{c c@{\hspace{0.2mm}} c@{\hspace{0.2mm}} c}
    
    % Legend.
    % Note: first column is rotated sequence title

    &
    \seqDynamicFace &
    \seqJumping
    \\
    %%%%%%%%%%%%%%%%%%%%%%%%%
    % Sequence: Features

    % Labels
    %&
    %Balloon1-2 &
    %Balloon2-2 &
    %DynamicFace-2 & 
    %Jumping &
    %Umbrella
    %\\    

    \rotatebox{90}{\hspace{0.6cm} Input} &
     
    % \imgRGB[45px 0px 0px 0px]{\figSeqTwoDim/ezgif-frame-001.jpeg} &
    %\imgRGB[45px 0px 0px 0px]{\figSeqBalloon/00000.png} &

    %\imgRGB[100px 0px 0px 0px]{\figSeqVolume/ezgif-frame-001-render.jpeg} &
    %\imgRGB[45px 0px 0px 0px]{\figSeqBalloonw/00000.png} &

    %\imgAtt[34px 0px 0px 0px]{\figSeqTwoDim/ezgif-frame-001-sal.png} &    
    \imgRGB[45px 0px 0px 0px]{\figSeqDynamicFace/00015.png} &
    
    % \imgAtt[100px 0px 0px 0px]{\figSeqVolume/0_sal.png} 
    \imgRGB[45px 0px 0px 0px]{\figSeqJumping/00023.png} &
    
    % \imgAtt[100px 0px 0px 0px]{\figSeqVolume/0_sal.png} 
    %\imgRGB[45px 0px 0px 0px]{\figSeqUmbrella/00000.png} &
    \\

    % Images for pyramid preprocess
    %
    \rotatebox{90}{\hspace{0.7cm} Raw} &
     
    % \imgRGB[45px 0px 0px 0px]{\figSeqTwoDim/ezgif-frame-001.jpeg} &
    %\imgRGB[45px 0px 0px 0px]{\figSeqBalloon/00000.png} &

    %\imgRGB[100px 0px 0px 0px]{\figSeqVolume/ezgif-frame-001-render.jpeg} &
    %\imgRGB[45px 0px 0px 0px]{\figSeqBalloonw/00000.png} &

    %\imgAtt[34px 0px 0px 0px]{\figSeqTwoDim/ezgif-frame-001-sal.png} &    
    \imgRGB[45px 0px 0px 0px]{\figSeqDynamicFace/15_raw.png} &
    
    % \imgAtt[100px 0px 0px 0px]{\figSeqVolume/0_sal.png} 
    \imgRGB[45px 0px 0px 0px]{\figSeqJumping/23_raw.png} &
    
    % \imgAtt[100px 0px 0px 0px]{\figSeqVolume/0_sal.png} 
    %\imgRGB[45px 0px 0px 0px]{\figSeqUmbrella/00000.png} &
    \\

    %%%%%%%%%%%%%%%%%%%%%%%%%%%%%%
    % Sequence: Pyramid preprocess
    
    % Labels for pyramid preprocess
    \rotatebox{90}{\hspace{0.3cm} Post Processed} &
     
    % \imgRGB[45px 0px 0px 0px]{\figSeqTwoDim/ezgif-frame-001.jpeg} &
    %\imgRGB[45px 0px 0px 0px]{\figSeqBalloon/training_ 0.png} &

    %\imgRGB[100px 0px 0px 0px]{\figSeqVolume/ezgif-frame-001-render.jpeg} &
    %\imgRGB[45px 0px 0px 0px]{\figSeqBalloonw/training_ 0.png} &

    %\imgAtt[34px 0px 0px 0px]{\figSeqTwoDim/ezgif-frame-001-sal.png} &    
    \imgRGB[45px 0px 0px 0px]{\figSeqDynamicFace/15.png} &
    
    % \imgAtt[100px 0px 0px 0px]{\figSeqVolume/0_sal.png} 
    \imgRGB[45px 0px 0px 0px]{\figSeqJumping/23.png} &
    
    % \imgAtt[100px 0px 0px 0px]{\figSeqVolume/0_sal.png} 
    %\imgRGB[45px 0px 0px 0px]{\figSeqUmbrella/training_ 0.png} &
    \\

    \end{tabular}

    \vspace{-0.25cm}
    \caption{
        %\textbf{Post processing effect.} 
        Post processing helps remove small noisy regions from the raw results while maintaining thin features. 
    }
	
    \label{fig:postprocessed}
    \vspace{-0.25cm}
\end{figure}

}

% During object extraction, we also obtain the corresponding segmentation mask without setting the density to be zero. This tells us whether each pixel will be background in a particular view. After extracting the object and rendering 2D color images, we set the background pixels to be transparent.  

\paragraph{Optimization routine and hyperparameters}

We optimize the combined loss with Adam optimizer, learning rate $5e^{-4}$, $\beta=(0.9$, $0.999)$. We multiply prior losses for depth and optical flow by a decay rate. This rate starts at 1 and is divided by 10 at every 300,000$^{\text{th}}$ iteration.
%
% Code for decay scheme; optimization iteration i
% decay_iteration = 30
% divsor = i // (decay_iteration * 1000)
% decay_rate = 10
% if args.decay_depth_w:
%     w_depth = args.w_depth/(decay_rate ** divsor)
% else:
%     w_depth = args.w_depth
%
For \titlename, we set reprojection losses $\lambdaSAFFsemproj=1.0$ and $\lambdaSAFFattproj=1.0$, and prior losses $\lambdaSAFFsem=0.04$ and $\lambdaSAFFatt=0.04$~\cite{kobayashi2022distilledfeaturefields}. For all other losses, we follow Li et al.~\cite{li2020neural}:  %
$\lambdaNSFFRegFlowSmall = 0.1$,
$\lambdaNSFFRegFlowSmooth = 0.1$,
$\lambdaNSFFw = 0.1$,
$\lambdaNSFFPixColProj = 1.0$,
$\lambdaNSFFCyc = 1.0$,
$\lambdaNSFFd = 0.04$,
$\lambdaNSFFof = 0.02$,
$\lambdaNSFFentropy = 0.001$.

\titlename, its ablations, and NSFF are optimized for $360$k iterations. As \ddnerf is a different architecture, we use the author's stated $100$k iterations.

\paragraph{Computational cost.}
The code was developed on Ubuntu 20.10 in Python/PyTorch, and trained on NVIDIA GeForce RTX 3090, NVIDIA GeForce RTX A6000, and NVIDIA GeForce RTX 2080 TI GPUs. All operations assume access to only $1$ GPU. The CUDA VRAM required for using a trained \titlename on $540\times 288$ image size is $12$ GB, while optimization requires $24$ GB. 
% The minimum cuda memory required for using \titlename drops to $12$ GB when image size shrinks to $128*128$. 
The CPU RAM used to optimize, cluster, and render \titlename used $16$ GB, while we use $36$ GB to extract objects. 
Optimizing a \titlename for $360,000$ iterations takes $1$ to $2$ days, depending on hardware, and is similar in time to NSFF. Recent improvements have dramatically reduced this time for non-semantic-attention fields~\cite{muller2022instant,chen2022tensorf}, and we expect similar performance gains were these methods used as the underlying architecture. In terms of runtime, we preprocess the \semfeatnetwork features and so do not incur significant additional cost during optimization, and none during inference due to \semfeatnetwork. Per-frame rendering is 15\% slower than NSFF due to the additional heads. Saliency-aware clustering takes a few seconds only.

The computational cost is currently expensive, but we see our work as a step towards integrating high and low level information for 4D semantic volume reconstruction. NeRF-based approaches are still some way from real-time performance, but there have been significant gains recently (e.g., InstantNGP~\cite{muller2022instant}). Building our approach upon a fast backbone like this would make our approach more practical. One additional note is that, versus supervised 2D segmentation networks that are typically trained to be feed forward and to make predictions quickly (e.g., ProposeReduce takes only a few seconds to process a short sequence), the output of our model is richer as a 4D reconstruction with time-varying correspondence.

With respect to scalability, longer sequences will take more time to process, and at some point the capacity of the MLPs will limit reconstruction detail. For scenes with more dynamic elements, many objects are not in principle a problem, but instances that spatially overlap cannot be separately determined due to the fact that DINO-ViT features are not instance-aware.

\paragraph{Network architecture}
We add two heads to the architecture of NSFF~\cite{li2020neural}. For the semantic head, we add a single linear layer (256 neurons) appended by a tanh layer, with output dimension 64 to match the size of the per-sequence PCA-reduced \semfeatnetwork features. For the saliency head, we add a single linear layer (256 neurons) appended by a sigmoid layer, with output dimension 1. 

%\vspace{-0.15cm}
%\paragraph{Pseudocodes}
%We include the saliency-aware clustering (Alg.~\ref{alg:cluster}) and the pyramid construction (Alg.~\ref{alg:pyr_final}).

% \input{fig/fig_edits/fig_edits}

%%%%%%%%%%%%%%%%%%%%%%%%%%%%%%%%%%%%%
%
% \clearpage
% \section{Results with Complete Decompositions}

% \jt{Visualize color, depth, flow, in video.}

% \YL{Video}
% \YL{arxiv (really popular domain!)}

% \YL{website: don't need for now? cannot use brown domain anyways}

% \YL{show (edge) issues with other pyramid weight settings}

% \YL{show D2NeRF reconstruction issue}

% \YL{show decay}

% \YL{add reference to supplementary material again? as reference part changed }

%\clearpage
%\input{alg/alg_pyramid.tex}

%\clearpage
%\input{alg/alg_clustering.tex}
