# Supplementary material for: Semantic Attention Flow Fields for Monocular Dynamic Scene Decomposition
Source: arXiv:2303.01526 source file (2023-09-29)
Supplement: Supplementary file 2 [file tab_related_expanded_supplemental.tex]

{

\begin{table}
    \centering

    \newcommand{\yes}{\ding{51}}
    \newcommand{\no}{\ding{53}}
    \newcommand{\notapplicable}{N/A}
    
    \caption{
        An expanded comparison of related work in scene decomposition shows the unstudied area of real-world dynamic 3D segmentation without explicit segmentation clues. We investigate whether saliency can provide similar clues for the monocular video case. From this table, the closest related method is N3F; however, they take user input to define their segmentation.
       \\
        T: Large-scale task-specific. \\
        P: Generic pretraining.
        \label{tab:relatedwork_expanded}
    }
    %\resizebox{\linewidth}{!}{
    \begin{tabular}{l c c c  c c c c c }
    
    \toprule
    {} & \multirowcell{2}{Dynamic\\(video)} &
    \multirowcell{2}{Monocular} &
    \multirowcell{2}{Real\\world} & \multirowcell{2}{3D} & \multirowcell{2}{No seg. \\clue} &
    \multirowcell{2}{Learning} & 
    \multirowcell{2}{Adaptive \\ \# objects} &
    \multirowcell{2}{Object-\\level}\\
    \\
    \midrule
    
    IODINE\cite{greff2019multiobject} & \no & \yes & \no & \no & \yes & \no & \no & \yes\\
    MONET\cite{burgess2019monet} & \no & \yes & \no & \no & \yes & \no & \no & \yes\\
    Slot Attention\cite{locatello2020object} & \no & \yes & \no & \no & Mask & T & \no & \yes\\
    
    \midrule
    
    SIMONe\cite{Kabra2021SIMONeVT} & \yes & \yes & \no & \no & \yes & \no & \no & \yes\\
    SAVi\cite{kipf2022conditional} & \yes & \yes & \no & \no & Mask & T & \no & \yes\\
    SAVi++\cite{elsayed2022savipp} & \yes & \yes & \yes & \no & Mask & T & \no & \yes\\
    
    \midrule
    
    ObSuRF\cite{stelzner2021decomposing} & \no & \no & \no & \yes & \yes & \no & \no & \yes\\
    uORF\cite{yu2022unsupervised}& \no & \no & \no & \yes & \yes & \no & \no & \yes\\
    COLF\cite{smith2022colf} & \no & \no & \no & \yes & \yes & \no & \no & \yes\\
    
    \midrule
    
    PNF\cite{Kundu_2022_CVPR} & \yes & \yes & \yes & \yes & Mask & \no & \no & \yes \\
    %Panoptic-NeRF \cite{fu2022panoptic} & \yes & \yes & \yes & \no\\
    Object-NeRF \cite{yang2021objectnerf} & \no & \no & \yes & \yes & Mask & \no & \no & \yes\\
    
    \midrule
    DFF\cite{kobayashi2022distilledfeaturefields} & \no & \no & \yes & \yes & User & P & \yes & \yes\\
    N3F\cite{tschernezki22neural} & \yes & \yes & \yes & \yes & User & P & \yes & \yes\\
    
    \midrule
    ProposeReduce\cite{lin2021video} & \yes & \yes & \yes & \no & \yes & T & \yes & \yes\\
    NSFF\cite{li2020neural} & \yes & \yes & \yes & \yes & Mask & \no & \notapplicable & \notapplicable\\
    D$^2$NeRF\cite{wu2022ddnerf} & \yes & \yes & \yes & \yes & \yes & \no & \notapplicable & \notapplicable\\
    \midrule
    \titlename (this paper) & \yes & \yes & \yes & \yes & \yes & P & \yes & \yes\\
    
    \bottomrule
    
    \end{tabular}
    %}
\end{table}

}
